# Supplementary material for: Trion formation in a two-dimensional hole-doped electron gas
Source: arXiv:1505.07411 ancillary file (2016-08-10)
Supplement: Supplementary file 1 [file supplemental.pdf]

# Trion formation in a two-dimensional hole-doped electron gas: Supplemental Material

G. G. Spink,[1,2] P. López Ríos,[1] N. D. Drummond,[3] and R. J. Needs[1]

[1] *TCM Group, Cavendish Laboratory, University of Cambridge, 19 J. J. Thomson Avenue, Cambridge CB3 0HE, United Kingdom*

[2] *Department of Chemical Engineering, University of Chester, Thornton Science Park, Chester CH2 4NU, United Kingdom*

[3] *Department of Physics, Lancaster University, Lancaster LA1 4YB, United Kingdom*

(Dated: April 5, 2016)

## ADDITIONAL PLOTS, TABLES AND ANALYSIS OF THE QUANTUM MONTE CARLO RESULTS

### Electron-hole relaxation energy

The electron-hole relaxation energies plotted in the main body of the paper are tabulated in Table S1 for the systems studied. Additional details of the calculations are given later in this document.

The energy of the system formed by a hole and a low-density $N$-electron gas is approximately that of an $(N-2)$-electron gas plus the total energy of a trion plus the energy gained by immersing the trion in the homogeneous electron gas (HEG),

$$E_{h+\mathrm{HEG}(N)} \approx E_{\mathrm{HEG}(N-2)} + E_{X^-} + E_{X^-}^{\mathrm{imm}} . \tag{S1}$$

From the vantage point of a low-density homogeneous electron gas (HEG), a tightly bound trion is similar to an electron of overall charge $-1$, and in this limit $E_{X^-}^{\mathrm{imm}}$ is approximately equal to the Fermi energy of the HEG, $E_F$, which for an infinite 2D HEG is

$$E_F = \epsilon(r_s) - \frac{r_s}{2}\frac{d\epsilon(r_s)}{dr_s} , \tag{S2}$$

where $\epsilon$ is the energy per electron as a function of HEG density parameter $r_s$. Therefore the relaxation energy is

$$\begin{aligned} E_R &= E_{h+\mathrm{HEG}(N)} - E_{\mathrm{HEG}(N)} \\ &\approx -2E_F + E_{X^-} + E_{X^-}^{\mathrm{imm}} \\ &\approx -E_F + E_{X^-} . \end{aligned} \tag{S3}$$

At high densities the delocalized nature of the collective excitonic state prevents a simple analysis similar to that for the low-density regime. Based on the analytical high-density limit of the relaxation energy in three dimensions given in Ref. [1], at $r_s \to 0$ we expect $E_R$ to diverge towards $-\infty$ at a slower rate than $-E_F$. See below for a physical explanation of the divergence of $E_R$ in terms of the behavior of the electron-hole PCF.

The difference between the relaxation energy and the isolated trion energy is shown in Fig. S1, along with the Fermi energy of the HEG obtained using the parameterization of $\epsilon(r_s)$ given in Ref. [2]. The difference between the relaxation energy and the isolated trion energy approaches $-E_F$ at low density, while the high density behavior is qualitatively similar to that in three dimensions.

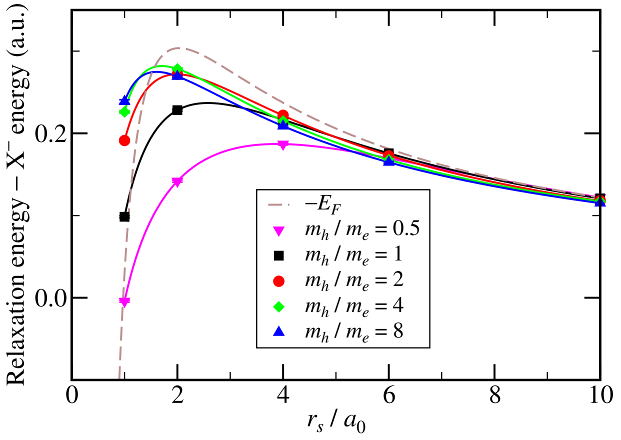


FIG. S1. Difference between relaxation energy and isolated trion energy. The dashed line is the negative of the Fermi energy of the HEG, calculated using the results of Ref. [2], for comparison. Note that, in contrast to the similar Fig. 1 in the main paper, atomic units are used on both axes here.

### Pair-correlation functions

#### *On-top pair density*

We replot our on-top pair-correlation function (PCF) data against the density parameter of the electron gas $r_s$ and reduced electron-hole mass $\mu$ in Fig. S2. The logarithmic scales used on both axes reveal an almost linear relationship between the logarithms of the on-top pair density and both $r_s$ and $\mu$. We now try to make sense of these patterns by adapting a well-known approximation to the electron-hole PCF for a neutral exciton in the limit of a dilute electron gas (see, e.g., Zhu *et al.* [3]).

By definition, the expected number of electrons within an annulus a distance $r$ from the hole and thickness $dr$ is $dN = 2\pi r n_e g_{eh}(r)\, dr$, where $n_e$ is the electron number density and $g_{eh}(r)$ is the electron-hole PCF. If the system consisted only of one electron and one hole in a bound, neutral exciton state, then the problem would be analogous to a hydrogen atom. A separation of variables leads to plane-wave center-of-mass motion together with a wave function in the relative coordinate (the distance between the two particles) given by the solution to the

TABLE S1. Electron-hole relaxation energies in a.u. for the densities and mass ratios studied. These results were obtained using diffusion Monte Carlo simulations of systems containing 86 electrons, as described in the text.

| $r_s$ (a.u.) | $m_h/m_e$ | | | | |
|---|---|---|---|---|---|
| | 0.5 | 1.0 | 2.0 | 4.0 | 8.0 |
| 1.0 | −0.763(1) | −1.023(1) | −1.295(1) | −1.556(2) | −1.745(2) |
| 2.0 | −0.617(1) | −0.893(1) | −1.214(1) | −1.504(1) | −1.714(1) |
| 4.0 | −0.572(1) | −0.905(1) | −1.264(1) | −1.567(1) | −1.775(1) |
| 6.0 | −0.589(1) | −0.946(1) | −1.314(1) | −1.614(1) | −1.819(1) |
| 10.0 | −0.637(1) | −1.001(1) | −1.368(1) | −1.665(1) | −1.868(1) |

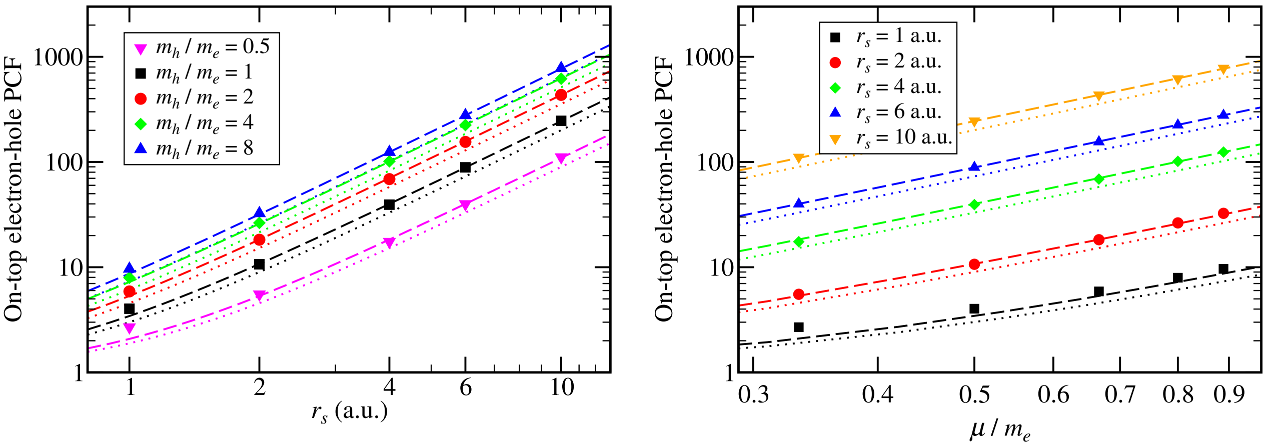


FIG. S2. On-top electron-hole PCFs for the systems studied plotted against the density parameter $r_s$ of the electron gas (left) and against the reduced mass of the electron-hole pair (right). Symbols denote the quantum Monte Carlo data; dotted lines show the neutral exciton in dilute gas limit [Eq. (S9) with $c = 8$]; and dashed lines show the fit [Eq. (S9) with $c = 9.742(7)$]. Error bars are smaller than the size of the symbols. Note the logarithmic scales on the axes.

hydrogen atom in two dimensions: a "particle" of mass $\mu$ in an attractive Coulomb potential. The normalized ground-state wave function of the 2D hydrogen atom is [4]

$$R_{nl} = R_{10} = \frac{4\mu}{\sqrt{2\pi}} \exp\left(-2\mu r\right) , \quad \text{(S4)}$$

in atomic units and for particles of unit charge.

The expected electron weight around the hole from this neutral exciton is $2\pi r|R_{10}|^2\, dr$. In addition there is a contribution from the dilute electron gas, which we model as an uncorrelated electron density contributing $2\pi r n_e\, dr$ to the electron weight around the hole since, in an uncorrelated gas, $g_{eh}(r) = 1$. Summing these contributions we get

$$dN = 2\pi r|R_{10}|^2\, dr + 2\pi r n_e\, dr = 2\pi r n_e g_{eh}(r)\, dr , \quad \text{(S5)}$$

which gives

$$g_{eh}(r) = 8\mu^2 r_s^2 e^{-4\mu r} + 1 . \quad \text{(S6)}$$

We anticipate the formation of negative trions at low electron density in a system with only one hole [5]. In a simple, independent-electron picture of the trion the two electrons would occupy the hydrogenic ground state, and the PCF for a trion in an electron gas would be similar to that of the exciton,

$$g_{eh}(r) = 16\mu^2 r_s^2 e^{-4\mu r} + 1 . \quad \text{(S7)}$$

Therefore we propose that the electron-hole PCF function for the trion immersed in an electron gas can be approximated by the following functional form,

$$g_{eh}(r) = c\mu^2 r_s^2 e^{-4\mu r} + 1 , \quad \text{(S8)}$$

where $c$ is a prefactor that we expect to vary slowly with density and reduced mass. The limit $c = 16$ of Eq. (S7) corresponds to a trion with two independent electrons in the hydrogenic ground state, but it is known that, in fact, the second electron in the negative hydrogen ion occupies a much more diffuse orbital [6], and therefore we expect that $c$ will be significantly less than 16, while also greater than the exciton limit of $c = 8$.

Setting $r = 0$ in Eq. (S8) gives the on-top pair density,

$$g_{eh}(0) = c\mu^2 r_s^2 + 1 , \quad \text{(S9)}$$

A fit of our quantum Monte Carlo (QMC) PCF data to Eq. (S9) yields a value of $c = 9.742(7)$. We analyze the variability of $c$ with $m_h/m_e$ and $r_s$ in Table

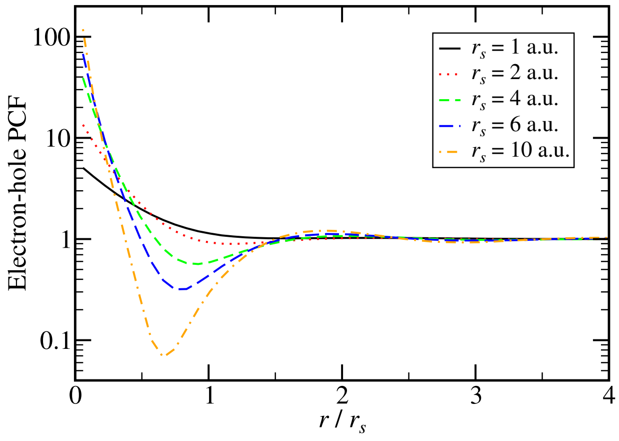


FIG. S3. Electron-hole PCFs for $m_h/m_e = 2$ over the range of densities studied. Note the logarithmic scale on the vertical axis.

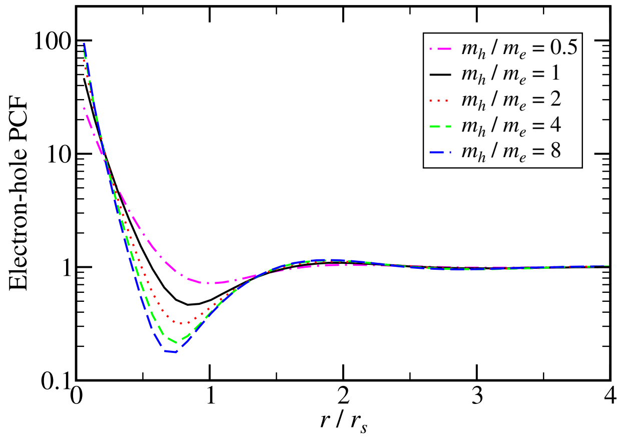


FIG. S4. Electron-hole PCFs for $r_s = 6$ a.u. over the range of mass ratios studied. Note the logarithmic scale on the vertical axis.

S2. The greatest deviation from $c = 9.742(7)$ occurs for $r_s = 1$ a.u., which is to be expected since we assume a dilute electron gas in our above derivation.

### *Complete PCFs*

We plot the full electron-hole PCFs as a function of $r/r_s$ for $m_h/m_e = 2$ over the range of densities we have studied in Fig. S3, and for $r_s = 6$ a.u. over the range of mass ratios used in our calculations in Fig. S4. In Fig. S5 we plot the integrated electron-hole PCFs as a function of $r$ for $m_h/m_e = 2$ and $m_h/m_e = 8$ at various densities. It can be seen that the short-range behavior of the PCFs is determined by the mass ratio while the long-range PCF is governed by the electron density. In exciton units (not shown) the small-$r$ regions of the curves for different mass ratios coincide, although the large-$r$ behavior then depends, albeit trivially, on mass ratio as well as electron density.

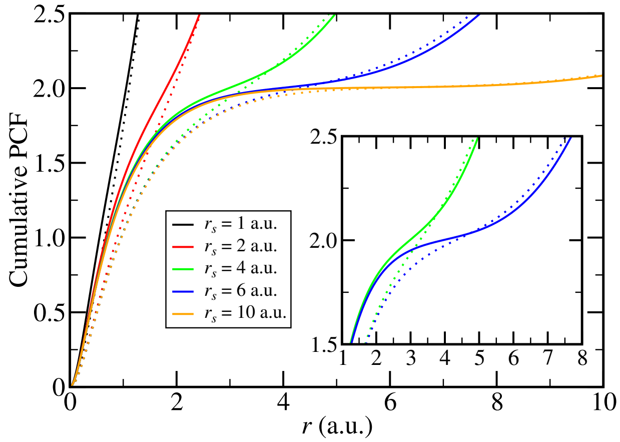


FIG. S5. Integrated electron-hole PCFs for $m_h/m_e = 2$ (dotted lines) and $m_h/m_e = 8$ (solid lines) at the densities studied. The inset shows data for $r_s = 4$ a.u. and $r_s = 6$ a.u. in the region that shows a crossover between short-range behavior determined by the mass ratio and long-range behavior determined by the electron density. Note that the horizontal axis is not scaled by $r_s$.

### *Connection between relaxation energy and $g(0)$*

It is interesting to contrast the monotonic decrease of $g(0)$ as the electron density rises with the behavior of the relaxation energy. Hodges and Stott [7] derive a relationship between the electron–hole PCF as a function of impurity charge $Z$, $g_{eh}(r, Z)$, and the relaxation energy $E_R$. In two dimensions, the relationship becomes

$$E_R = -\frac{2}{r_s^2} \int_0^1 dZ \int_0^\infty dr \, [g_{eh}(r, Z) - 1] \ . \tag{S10}$$

After restoring the $Z$-dependence of the hydrogenic orbitals of Ref. [4], the independent-electron approximation of Eq. (S8) reads $g_{eh}(r, Z) = 16\mu^2 Z^2 r_s^2 e^{-4\mu Z r} + 1$. Substitution into Eq. (S10) yields a constant relaxation energy of $E_R = -c/2$ Ry$^*$, which for the value $c = 9.742(7)$ results in $E_R = -4.871(3)$ Ry$^*$, in qualitative agreement with the range of the relaxation energies we report.

This independent-electron model cannot account for the $r_s$-dependence seen in the relaxation energy data, for example the increase in magnitude at high density, and it is the deviations of the PCF from this simple model that cause this behavior via the Hodges and Stott relation. Although the PCFs smoothly approach unity, the decay at high density is not rapid enough to keep pace with the $r_s^{-2}$ factor in Eq. (S10). Small deviations from the model are visible in the high density region of the on-top

TABLE S2. Prefactor $c$ in Eq. (S9) for each individual system studied. Fitted values of $c$ for each $m_h/m_e$ and each $r_s$ can be found in the "Fit" row and column, respectively, and the value obtained by fitting the data for all the systems studied is in the bottom-right cell.

| $r_s$ (a.u.) | $m_h/m_e$ | | | | | |
|---|---|---|---|---|---|---|
| | 0.5 | 1.0 | 2.0 | 4.0 | 8.0 | Fit |
| 1.0 | 15.2(5) | 12.1(2) | 11.0(2) | 10.9(1) | 10.94(8) | 11.16(6) |
| 2.0 | 10.19(9) | 9.7(1) | 9.71(8) | 9.92(7) | 9.97(7) | 9.90(4) |
| 4.0 | 9.27(4) | 9.58(8) | 9.53(1) | 9.81(7) | 9.74(3) | 9.59(2) |
| 6.0 | 9.71(3) | 9.77(7) | 9.64(5) | 9.70(4) | 9.73(2) | 9.72(1) |
| 10.0 | 9.92(2) | 9.80(4) | 9.75(3) | 9.65(1) | 9.84(2) | 9.737(9) |
| Fit | 9.79(1) | 9.68(1) | 9.73(2) | 9.84(3) | 9.77(2) | 9.742(7) |

PCFs shown above and in the main paper, where it is seen that the QMC data do not decay quite as rapidly with increasing density as predicted.

In addition, the model does not describe the exchange-correlation hole around the trion, although this is only significant at low density. Since the low-density HEG perceives the trion as an object similar to an electron, an exchange-correlation hole develops around the trion, which is not included in the simple model presented.

*Screening charge*

The charged impurity is screened by an equal charge drawn away from the bulk electron gas. If the electron density far from the hole is $n$ and the electron density as a function of position is $n(r)$, the induced screening charge within a thin spherical shell centered on the hole is $[n(r) - n]2\pi r\,dr = \Delta n(r)2\pi r\,dr$. This screening charge density is obtained from the electron-hole PCF via $\Delta n(r) = n\,[g_{eh}(r) - 1]$. We know that $\int \Delta n(r)2\pi r\,dr = Z$, with $Z$ the charge on the impurity, and from Hodges and Stott that $E_R = -\int dZ \int \frac{\Delta N(r)}{r} 2\pi r\,dr$.

We show in Fig. S6 the integrated (cumulative) additional electron weight drawn around the hole in order to screen it, $\int_0^r \Delta n(r')2\pi r'\,dr'$, for systems with hole mass $m_h = 0.5$ a.u. and the range of carrier densities studied. An additional test calculation at $r_s = 0.5$ a.u. is also shown to clarify the behavior at high density. The total electron weight drawn in is one unit of charge for all systems. The short-range screening charge is insensitive to carrier density above $r_s \gtrsim a_0^*$, but at higher densities the screening electron weight moves closer to the hole, giving rise to a rapid increase in the magnitude of the relaxation energy in the Hodges and Stott formula, as seen in the QMC data. Friedel oscillations can be seen at lower densities.

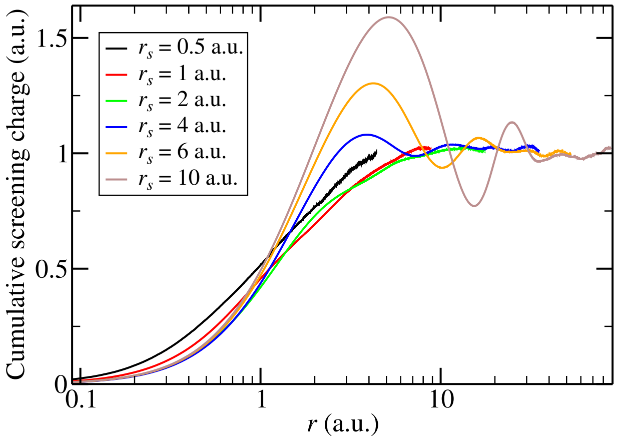


FIG. S6. Integrated (cumulative) additional electron weight within radius $r$ of the hole due to screening for hole mass $m_h = 0.5$ a.u. over the full range of carrier densities studied, along with an additional test calculation at $r_s = 0.5$ a.u. to show the trend at high density.

*Minima in electron-hole PCFs*

In the main paper we show the gradual crossover between the collective excitonic state and the localized trion state using the minima in the electron-hole PCFs, effectively comparing the minimum electron density to that far from the hole. Similar results can be obtained by analyzing the minimum electron density around the hole in absolute terms. The electron density is $ng(r)$, where $n$ is the density of the electron gas far from the hole. The minimum of this quantity is plotted against $r_s$ in Fig. S7. The minimum density around the hole falls below the density corresponding to one electron in a circle of radius $a_0^*$ (which is $1/\pi$ in excitonic units) close to $r_s \sim a_0^*$. By $r_s \sim 4\,a_0^*$, the electron density is less than 1% of this reference density. Features associated with isolated excitonic species are therefore expected to emerge in absorption spectra in this parameter range, consistent with the trends seen in all other expectation values reported in this work.

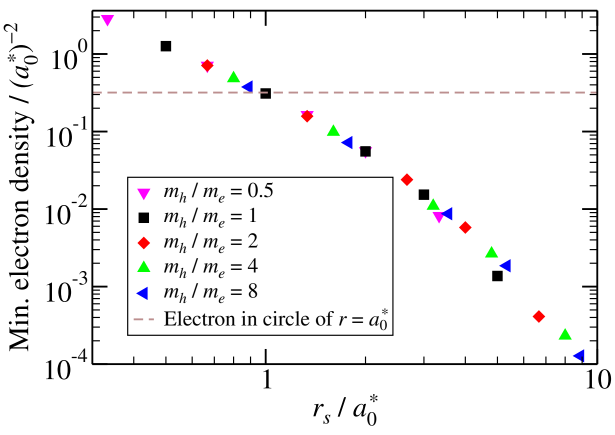


FIG. S7. Minimum electron density around the hole as a function of $r_s$ in all systems studied. The density corresponding to one electron in a circle of radius $a_0^*$ is also shown. Excitonic units are used.

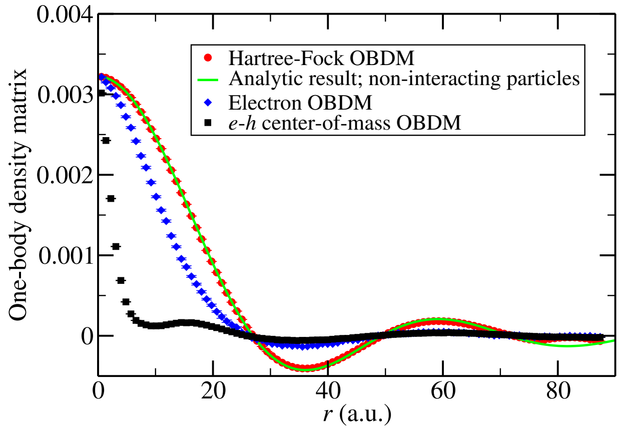


FIG. S8. One-body density matrix corresponding to the momentum density for the electron-hole pair with $m_h/m_e = 8$ and $r_s = 10$ a.u. (black squares). Also displayed are the one-body density matrix for electrons (blue diamonds), the Hartree-Fock one-body density matrix (calculated with variational Monte Carlo using the Hartree-Fock wave function) and the analytical result for noninteracting electrons.

## Momentum density

The momentum densities that we obtain at high $r_s$ have an unusual peaked feature above the Fermi edge. This small peak appears to develop in those systems where trion-like features are present in the energies and PCFs. In contrast, a strong enhancement just below the Fermi edge, together with almost no weight above $k_F$ has been predicted analytically [8, 9], and observed numerically [10], for 3D systems in the high density regime of a correlated electron-hole plasma. We also observe this behavior at high density, which supports the interpretation that the high density systems we have studied form electron-hole plasmas. In the following, we try to rationalize the peaked feature we observe at low density by showing that it can be regarded as a trion-like feature. The clear differences in the momentum densities thus support the interpretation of a correlated plasma to trion crossover, as also suggested by the other expectation values.

The "electron-hole center-of-mass one-body density matrix"

$$\rho(\mathbf{r}) = \frac{N_e}{\Omega}\left\langle \frac{\Psi(\mathbf{r}_1+\mathbf{r};\mathbf{r}_1+\mathbf{r},\mathbf{r}_2,\ldots,\mathbf{r}_{N_e})}{\Psi(\mathbf{r}_1;\mathbf{r}_1,\mathbf{r}_2,\ldots,\mathbf{r}_{N_e})}\right\rangle , \quad \text{(S11)}$$

where angled brackets denote averaging over the distribution $|\Psi(\mathbf{r_1};\mathbf{r_1},\mathbf{r}_2,\ldots,\mathbf{r}_{N_e})|^2$, is related by Fourier transform to the electron-hole center-of-mass momentum density. This quantity is shown in Fig. S8 for the system with $m_h/m_e = 8$, $r_s = 10$ a.u., where the trion-like features are strongest. For comparison, also displayed is the normal "electron" one-body density matrix, along with the Hartree-Fock result and the Fourier transform of the circular function, $J_1(r)/r$, which is the correct noninteracting behavior. The one-body density matrices are normalized so that $\rho(r = 0) = N_e/\Omega$.

The electron-hole center-of-mass one-body density matrix shows a large peak at the origin, followed by an additional local minimum before rising slightly to oscillate in the usual way. These features can be understood intuitively as being associated with a trion state because the wave function is then strongly peaked around the hole with an exchange-correlation hole induced by the trion, as seen in the electron-hole PCFs at low density.

The unusual feature in the momentum density above $k_F$ is consistent with this distinctive behavior in real space. Consider a hypothetical one-dimensional system and the following Gaussian model of a similar feature in the momentum density

$$f(\bar{k}) = \frac{1}{\sqrt{2\pi\sigma_{\bar{k}}^2}}e^{-(\bar{k}-k_B)^2/2\sigma_{\bar{k}}^2} + \frac{1}{\sqrt{2\pi\sigma_{\bar{k}}^2}}e^{-(\bar{k}+k_B)^2/2\sigma_{\bar{k}}^2} . \quad \text{(S12)}$$

We label the center of the feature in $\bar{k}$-space by $k_B$ and its width by $\sigma_{\bar{k}}$. We plot only the magnitude of $\bar{\mathbf{k}}$ in our momentum densities but the symmetry in $\bar{k}$-space is important when calculating the Fourier transform and, in one dimension, we must also include the peak at $-k_B$; in two dimensions, the feature is circularly symmetric, as discussed below. The one-dimensional Fourier transform of the above contribution to the momentum density is

$$f(x) = \sqrt{\frac{2}{\pi}}\cos(k_B x)e^{-\sigma_{\bar{k}}^2 x^2/2} . \quad \text{(S13)}$$

This gives a strong enhancement of the peak at $x = 0$ in relation to the rest of the function and can create a local

minimum close to $x \sim \pi/k_B$. (To avoid confusion, we use $x$ as the real-space coordinate in this one dimensional system.)

The situation in two dimensions is qualitatively similar, although the integrals cannot be evaluated analytically. We work with circularly symmetric functions and therefore need only consider the variation with the magnitude of $\bar{\mathbf{k}}$ or $\mathbf{r}$. Consider again a simple Gaussian model of the feature in the momentum density

$$f(\bar{k}) = \frac{1}{\sqrt{2\pi\sigma_{\bar{k}}^2}} e^{-(\bar{k}-k_B)^2/2\sigma_{\bar{k}}^2} . \tag{S14}$$

The two-dimensional Fourier transform of this function is

$$f(r) = \int_0^\infty \frac{1}{\sqrt{2\pi\sigma_{\bar{k}^2}}} e^{-(\bar{k}-k_B)^2/2\sigma_{\bar{k}}^2} \bar{k} J_0(r\bar{k}) d\bar{k} , \tag{S15}$$

where $J_n$ represents the $n^{\rm th}$-order Bessel function. A simple approximation can be obtained in the limit $\sigma_{\bar{k}} \to 0$ when the Gaussian becomes a delta function and $f(r) = k_B J_0(k_B r)$. We have also numerically evaluated the integral for values of the parameters $k_B$ and $\sigma_{\bar{k}}$ that more accurately represent the feature in the momentum density to confirm that this crude approximation is qualitatively correct up to the first minimum, although the finite width of the feature forces the oscillations of the Bessel function to decay far more rapidly as $r$ increases. The contribution to the one-body density matrix is again an enhancement at $r = 0$ and the possible creation of a local minimum around $r \sim j_{1,1}/k_B$, where $j_{1,1} \approx 3.8317$ is the first minimum of the zeroth order Bessel function.

The unusual feature in the momentum densities above $k_F$ found at low density corresponds to the distinctive features seen in the one-body density matrix at low density: a large peak at $r = 0$ and an additional local minimum, which are not seen at high density but gradually appear as the density is lowered. This behavior can be understood intuitively from the electron-hole PCFs, which shows that the wave function is sharply peaked around the hole and develops an increasingly pronounced exchange-correlation hole as the density decreases. We therefore interpret the evolution of the momentum densities as consistent with a crossover from a collective excitonic state to a trion immersed in a HEG.

Although the precise form of the momentum density is very sensitive to the details of the wave function, the simple picture above can explain qualitatively the trends seen in the numerical data. As the density is lowered, the feature becomes more pronounced as weight shifts from the states below $k_F$, which will further emphasize the expected trion-like behaviors seen in the low density one-body density matrix. The center of the feature in the momentum density is approximately located at $k_B \sim A/r_{XC}$, where $r_{XC}$ is the radius of the exchange-correlation hole seen in the electron-hole PCFs and $A \approx 4$ is a constant whose value is consistent with the derivation above. The peak in $\bar{k}$-space becomes narrower at lower density, which gives a more pronounced local minimum in the one-body density matrix, as expected.

### Isolated trion energies

The diffusion quantum Monte Carlo (DMC) energies of the isolated trion used in the main body of the paper are given in Ry* in Table S3 as a function of $m_h/m_e$. These data are extrapolated to zero time step and population control bias was verified to be negligible. The DMC method is exact for these systems because there is no nodal surface in their respective ground-state wave functions. Note that the energy of a positive trion $X^+$ is equal to that of the negative trion at the inverse mass ratio: $E_{X^+}(m_e/m_h) = E_{X^-}(m_h/m_e)$.

TABLE S3. Isolated negative trion ($X^-$) total energies for the mass ratios studied. For reference, the total energy of an exciton is $E_X = -4$ Ry* at all mass ratios.

| $m_h/m_e$ | $E_{X^-}$ (Ry*) |
|---|---|
| 0.0 | −5.64475(2) |
| 0.0625 | −4.9687(3) |
| 0.125 | −4.8112(2) |
| 0.25 | −4.66654(8) |
| 0.5 | −4.55453(2) |
| 1.0 | −4.48637(1) |
| 2.0 | −4.45853(2) |
| 4.0 | −4.45593(2) |
| 8.0 | −4.46266(1) |
| 16.0 | −4.46973(2) |
| $\infty$ | −4.48057(1) |

We have fitted the negative trion energies to the following expansion in $\mu/m_e$,

$$E_{X^-} \approx k_0 + k_1 (\mu/m_e)^{1/2} + k_2 \mu/m_e + k_3 (\mu/m_e)^{3/2} + k_4 (\mu/m_e)^2 , \tag{S16}$$

where $k_i$ are fitting parameters whose values are given in Table S4. Equation (S16) is motivated by the fact that the Born-Oppenheimer approximation is applicable when $m_h/m_e$ is small and that, furthermore, the Born-Oppenheimer interelectronic potential may be approximated by a harmonic potential when $m_h/m_e$ is very small. The zero-point energy of this harmonic oscillator gives the leading-order $m_h/m_e$-dependence, which goes as $\sqrt{m_h/m_e}$. By contrast, when $m_h/m_e$ is large, the system resembles a two-dimensional $H^-$ ion. The leading-order dependence on the mass ratio comes from the mass-polarization correction to the energy, which goes as $m_e/m_h$. Equation (S16) satisfies both these limits.

TABLE S4. Fitting parameters in Eq. (S16) for the total energy of the negative trion, with error bars computed from the least-squares fit.

| Parameter | Value (Ry*) |
|---|---|
| $k_0$ | $-5.64476(2)$ |
| $k_1$ | $3.8445(12)$ |
| $k_2$ | $-5.1318(46)$ |
| $k_3$ | $3.7943(59)$ |
| $k_4$ | $-1.3428(25)$ |

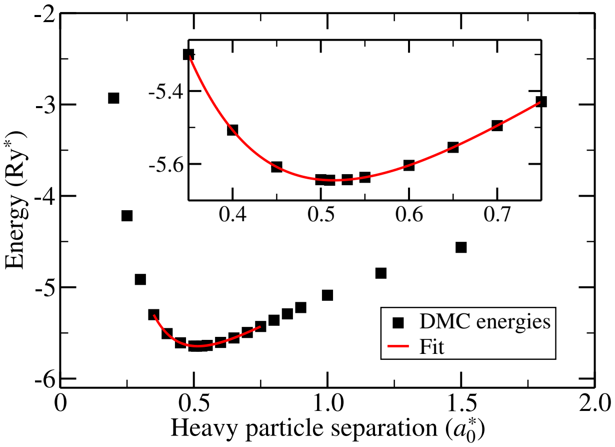


FIG. S9. DMC energy (squares) as a function of electron separation in the $m_h/m_e = 0$ negative trion. The line shows the fit of Eq. (S17) used to find the equilibrium separation. As shown, DMC energies over a range of separations from $0.35\,a_0^*$ to $0.75\,a_0^*$ were used in the fit. Error bars on the location of the minimum were obtained by a Monte Carlo bootstrap procedure. Error bars on the DMC data are smaller than the size of the symbols.

Obtaining the $m_h/m_e = 0$ limit required optimizing the heavy particle separation, as infinite-mass particles are fixed in space. This was done by evaluating the DMC energy over a range of particle separations and locating the equilibrium position using a fit to the data near the minimum of the form

$$E(d) = \frac{k_0 + k_1 d + k_2 d^2}{1 + k_3 d + k_4 d^2} \, . \tag{S17}$$

The data and fit are displayed in Fig. S9. A Monte Carlo bootstrap procedure was used to obtain error bars on the position of the minimum, resulting in the value $0.51454(2)\,a_0^*$.

## ADDITIONAL TECHNICAL DETAILS OF THE QUANTUM MONTE CARLO CALCULATIONS

### Diffusion Monte Carlo time step and target population

There are three physically significant length scales in the finite-size model of the hole-in-HEG systems: the exciton Bohr radius, $r_s$, and the linear size of the simulation cell. The smallest length scale is usually the exciton Bohr radius (although $r_s$ is smaller at the highest density we have studied) and this must therefore guide our choice of DMC time step.

Our hole-in-HEG DMC calculations were performed with time steps ranging from 0.005–0.05 a.u. The resulting acceptance ratios were usually higher than 99% for the electrons and always greater than 98% for both the hole and electrons. The increase in cell size as the density is lowered (and the constancy of the exciton Bohr radius) mean that the simulations necessarily take longer to explore configuration space. Larger time steps are permissible for the HEG calculations at low density, and we used up to 0.8 a.u., with corresponding acceptance ratios higher than 99%. In all cases, linear time step extrapolation was used and we verified in three test cases that the time steps used were within the range where the DMC energy is linear in the time step.

Tests showed population bias was small at the production target population of 1024 configurations.

### Choice of trial wave function and system size

We have used novel pairing orbitals in our trial wave function in order to improve accuracy and reduce noise. Our pairing orbitals include an orbital-dependent electron-hole Jastrow function $u_G$ and an orbital-dependent electron-hole backflow function $\eta_G$, with

$$u_G(r) = \left(1 - \frac{r}{L_{u,G}}\right)^C \Theta(r - L_{u,G}) \sum_{l=0}^{n_u} c_{G,l} r^l \, , \tag{S18}$$

where $C$ is an integer truncation order, $\Theta$ is the Heaviside step function, $n_u$ is the expansion order, and $L_{u,G}$ and $c_{G,l}$ are optimizable parameters, and

$$\eta_G(r) = \left(1 - \frac{r}{L_{\eta,G}}\right)^C \Theta(r - L_{\eta,G}) \sum_{l=0}^{n_\eta} d_{G,l} r^l \, , \tag{S19}$$

where $n_\eta$ is the expansion order and $L_{u,G}$ and $d_{G,l}$ are optimizable parameters. The functions in Eq. (S18) and (S19) are smoothly truncated at optimizable distances $L_{u,G}$ and $L_{\eta,G}$ which are constrained to be less than or equal to the radius of the largest circle that can be inscribed within the Wigner-Seitz cell. To avoid redun-

dancy, we set $u_0 = 0$, as one of the $u_G$ functions factorizes out and can be absorbed into the global Jastrow factor. The pairing orbitals are constrained to be cuspless at electron-hole coalescence points and the electron-hole cusp condition is enforced via the Jastrow factor of Eq. (1) in the main paper [11]. We have used a simulation-cell Bloch vector of $\mathbf{k}_s = \mathbf{0}$ throughout.

We now describe comparisons between the results obtained with the optimized orbitals and those obtained using the standard plane-wave orbitals normally used in QMC studies of fluid phases of electron-gas systems for two test cases. In each case, an optimized Jastrow factor and an optimized backflow transformation, as described in the main text, were used. Tables S5 and S6 show that most improvement was obtained using the optimized orbitals at the variational Monte Carlo (VMC) level, although the VMC and DMC results were similar, suggesting that the fixed-node approximation has not significantly affected our final results. The pairing orbitals offer a superior description of the behavior of the particles near the impurity in VMC calculations. The fraction of the correlation energy recovered by the optimized orbitals becomes smaller as the system size increases, because the effect of the impurity diminishes compared to the bulk of the system. The fraction of the remaining DMC electron-hole relaxation energy recovered by the optimized orbitals in the VMC calculations remains approximately constant, however, although the wave functions can become harder to optimize as the system size increases.

The optimized orbitals require more parameters to be optimized: our wave functions for systems containing 86 electrons (and the hole) contained about 130 optimizable parameters, of which about 30 were in the Jastrow factor, about 30 were in the backflow transformation, and about 70 came from the optimized orbitals. Typically the VMC and DMC calculations took about three times longer using the more complicated orbitals, for a given number of time steps.

Finite-size effects are probably the most important limitation of our work. We examined the effects of changing the system size in two points of parameter space: $m_h/m_e = 1$ and $r_s = 2$ a.u.; and $m_h/m_e = 8$ and $r_s = 6$ a.u. In Figs. S10, S11, S12, and S13 we plot all of the quantities studied in this work for both test cases at a range of system sizes. Our energies show some variation with system size due to the quasi-random effect of momentum quantization, but the effects of this are small. The uncertainties due to system size in our relaxation energies are about 0.01 a.u. in both cases. The PCFs are well converged with respect to system size. It can be seen that noise during optimization seems to be more significant for the momentum density than system size.

**Calculating the electron-hole relaxation energy, PCF, and momentum density**

The electron-hole relaxation energy, which could also be described as the electron-hole correlation energy, is the difference $E_R = E_h - E_0$, where $E_h$ is the total energy of $N_e$ electrons and one hole in area $A$ and $E_0$ is the energy of a HEG containing the same number of electrons in the same area but without the hole [12]. We used $A = (N_e - 1)\pi r_s^2$ in all our calculations to reduce finite-size effects: the hole will draw on average one neutralizing electron from the surrounding electron gas away from the bulk, reducing the density of the electron gas in a finite simulation cell. Our choice of cell area ensures that the density of electrons far from the hole is correct [12, 13]. The trion binds two electrons to the hole but this in turn induces a neutralizing exchange-correlation hole, so that the long-range electron density is largely unaffected by the additional bound electron.

Electron-hole pair-correlation functions are evaluated by binning the electron-hole distances sampled as the simulation proceeds according to the definition

$$g_{eh}(r) = \frac{A}{2\pi r N_e} \left\langle \sum_{j=1}^{N_e} \delta(|\mathbf{r}_j - \mathbf{r}_h| - r) \right\rangle , \qquad \text{(S20)}$$

before performing a rotational and translational average. The DMC PCFs were well converged with respect to time step and so we averaged these, weighted by the inverse variances on the energies to account for the degree of statistical noise in each run, although the duration of the runs were also set so that the noise was very similar for each time step. Extrapolated estimation was used to remove the leading order dependence on the trial wave function: $g = 2g_{\rm DMC} - g_{\rm VMC}$, where $g_{\rm DMC}$ and $g_{\rm VMC}$ denote the DMC and VMC PCFs respectively, although our DMC and VMC data were very similar, confirming the quality of the trial wave functions used. To reduce finite-size effects in the electron-hole PCF, we account for the reduction of the long-range electron density by multiplying our $g_{eh}$ data by $N_e/(N_e - 1)$, so that the PCF approaches unity for large separations [12, 13].

The on-top PCF must be inferred by extrapolation of the data at finite particle separations. We fit a form compatible with Kimball's cusp conditions suggested by Drummond *et al.* [10] for the electron-hole PCF,

$$\ln g_{eh}(r) = a_0 - 4\mu r + a_2 r^2 + a_3 r^3 , \qquad \text{(S21)}$$

where $\mu$ is the reduced mass of the electron and hole, to our data for $r/r_s < 0.53$ (300 data points) for each system. The value of the on-top density is $g_{eh}(0) = \exp(a_0)$ and the uncertainty in this quantity was estimated by assigning a constant uncertainty $\sigma$ to the PCF data and setting its value so that $\chi^2 = \sum_i \left[g_{eh}^{(\rm fit)}(r_i) - g_{eh}(r_i)\right]^2/(d\sigma^2)$, where $d$ is the number

TABLE S5. Comparison of plane-wave and optimized orbitals for $m_h/m_e = 1$ and $r_s = 1$ a.u. We show the Hartree-Fock, VMC, and DMC energies for the systems containing the hole, along with the fractions of the DMC correlation energy recovered in these calculations, where the DMC result for optimized orbitals is taken as the exact energy, and VMC and DMC electron-hole relaxation energies. The on-top PCF data were extrapolated using VMC and DMC data obtained using the wave functions indicated. Atomic units are used where applicable.

| | Plane-wave orbitals | Optimized orbitals |
|---|---|---|
| Hartree-Fock energy (a.u./part.) | −0.0933779 | |
| VMC energy (a.u./part) | −0.212170(4) | −0.212408(3) |
| VMC relaxation energy (a.u.) | −0.9921(4) | −1.0128(4) |
| VMC variance (a.u.) | 0.882(9) | 0.687(1) |
| % corr. energy VMC | 99.224(8) | 99.423(8) |
| DMC energy (a.u./part.) | −0.21303(2) | −0.213099(9) |
| DMC relaxation energy (a.u.) | −1.017(2) | −1.023(1) |
| % corr. energy DMC | 99.95(1) | 100 |
| $g_{eh}(0)$ | 4.02(6) | 4.03(4) |

TABLE S6. As Table S5, but for $m_h/m_e = 8$ and $r_s = 10$ a.u.

| | Plane-wave orbitals | Optimized orbitals |
|---|---|---|
| Hartree-Fock energy (a.u./part.) | −0.0548998 | |
| VMC energy (a.u./part.) | −0.105238(4) | −0.105716(3) |
| VMC relaxation energy (a.u.) | −1.7914(3) | −1.8330(3) |
| VMC variance (a.u.) | 0.3917(3) | 0.194(1) |
| % corr. energy VMC | 97.81(2) | 98.74(2) |
| DMC energy (a.u./part.) | −0.10636(2) | −0.10636(2) |
| DMC relaxation energy (a.u.) | −1.868(2) | −1.868(1) |
| % corr. energy DMC | 99.99(4) | 100 |
| $g_{eh}(0)$ | 771.6(9) | 779(2) |

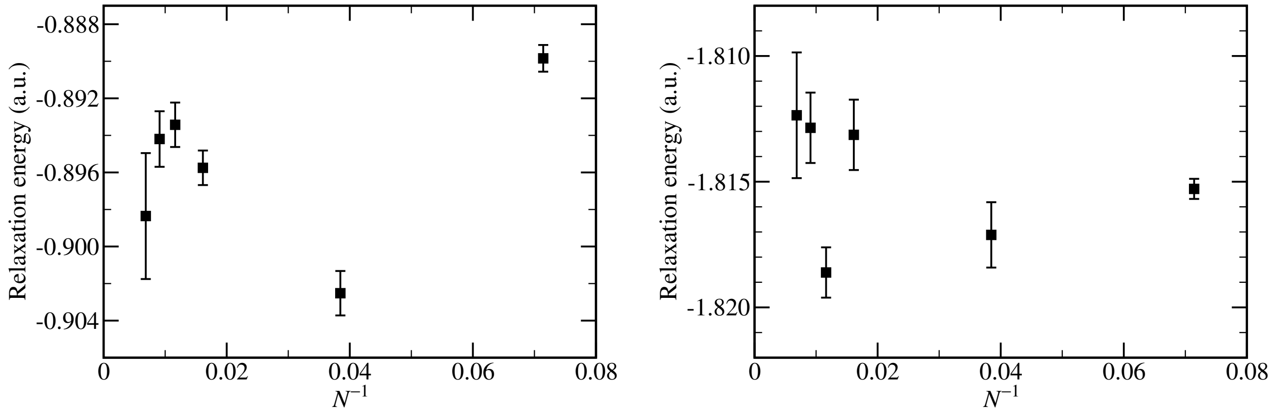


FIG. S10. DMC electron-hole relaxation energy against system size at $m_h/m_e = 1$ and $r_s = 2$ a.u. (left) and $m_h/m_e = 8$ and $r_s = 6$ a.u. (right).

of degrees of freedom, equals unity [10]. We assume four relations between the data (one each for the parameters estimated, together with one for the constraint that the observed frequencies in the bins sum to one) and therefore use $d = 300 - 4 = 296$ degrees of freedom.

We define an electron-hole center-of-mass momentum density $\rho$ following Drummond *et al.* [12] according to

$$\rho(\bar{\mathbf{k}}) = \left\langle \frac{1}{(2\pi)^2} \int \frac{\Psi(\mathbf{r};\mathbf{r},\mathbf{r}_2,\ldots,\mathbf{r}_{N_e})}{\Psi(\mathbf{r}_1;\mathbf{r}_1,\mathbf{r}_2,\ldots,\mathbf{r}_{N_e})} e^{i\bar{\mathbf{k}}\cdot(\mathbf{r}_1-\mathbf{r})}\, d\mathbf{r} \right\rangle , \quad \text{(S22)}$$

where the angled brackets denote an average over the

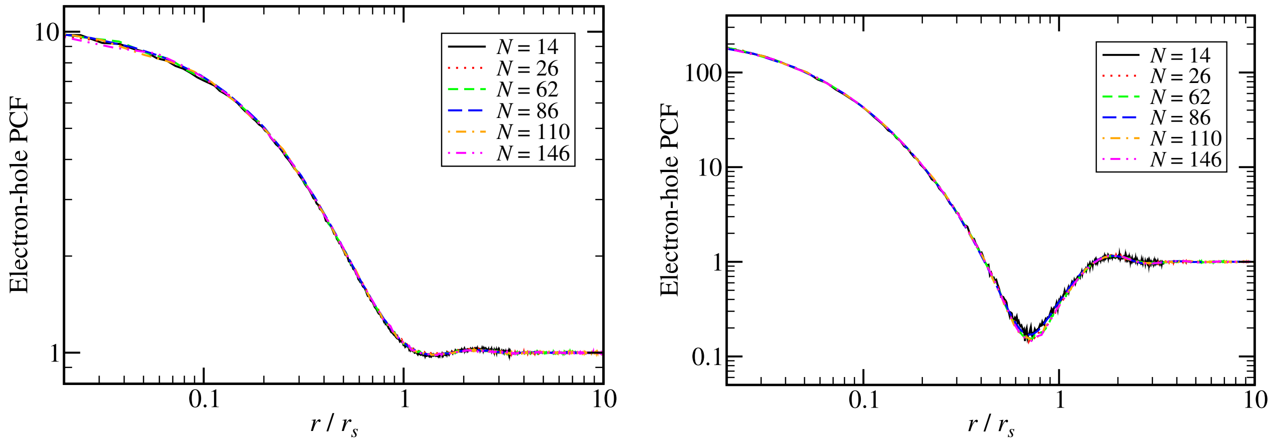


FIG. S11. Extrapolated electron-hole PCFs against $r/r_s$ at different system sizes at $m_h/m_e = 1$ and $r_s = 2$ a.u. (left) and $m_h/m_e = 8$ and $r_s = 6$ a.u. (right). Note the logarithmic scales on both axes.

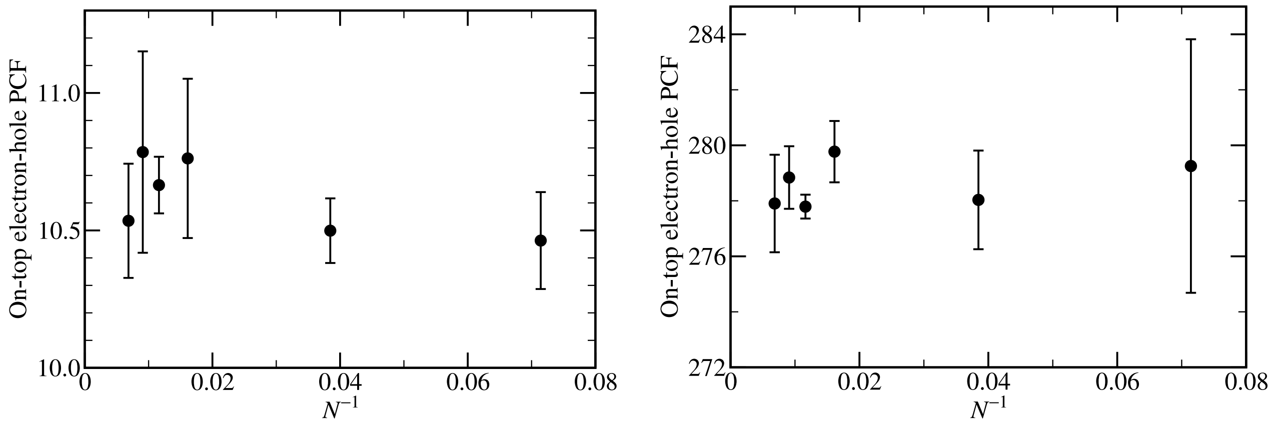


FIG. S12. On-top electron-hole PCFs against system size at $m_h/m_e = 1$ and $r_s = 2$ a.u. (left) and $m_h/m_e = 8$ and $r_s = 6$ a.u. (right).

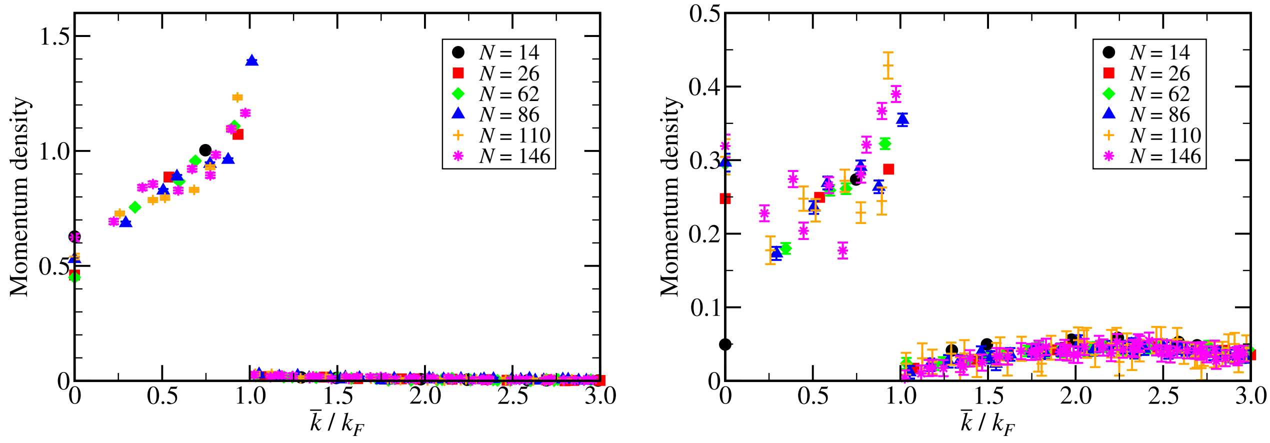


FIG. S13. Momentum densities at different system sizes at $m_h/m_e = 1$ and $r_s = 2$ a.u. (left) and $m_h/m_e = 8$ and $r_s = 6$ a.u. (right). The data shown here are calculated in VMC for wave functions optimized using 20,000 configurations and are not averaged over parameter sets from independent optimizations. The data are optimized and accumulated equivalently for each system size. The results shown for 86 electrons differ slightly from our best results (see text).

$N_e$-particle probability density obtained when an electron is constrained to be on top of the hole throughout

the simulation. This quantity can be evaluated in a VMC calculation with the constraint imposed on the configuration moves. The integral over $\mathbf{r}$ is accumulated as a Monte Carlo average at each time step.

The momentum density is very sensitive to the trial wave function and so we have carefully investigated the effects of noise during optimization. Initial optimizations were performed using 20,000 configurations during the energy minimization process. The VMC energies and PCFs so obtained were well behaved, but the momentum densities varied unpredictably from one optimized parameter set to another. To reduce the statistical noise during optimization, separate energy minimization runs were carried out using 500,000 configurations. In addition, eight independent optimized parameter sets were averaged to obtain the final results. For reasons of computational cost, we selected four representative systems to study using this procedure, as shown in the main paper. Here we further show the individual runs over which we averaged, alongside the original data for wave functions obtained using 20,000 configurations during optimization, and results obtained using plane-wave orbitals and backflow. We averaged eight independent runs for the final results (those optimized using 500,000 configurations) and six independent runs for the other two sets of data. The VMC energies and PCFs improved only a small amount when using the larger sample of configuration space although, as shown in Fig. S14, the effect on the momentum density was far more pronounced, at least below the Fermi edge. The difficulty of evaluating the momentum density with quantitative precision increases with $r_s$ and $m_h/m_e$.

## Material parameters

In order to compare the QMC data to experimental results, the dielectric constant and electron and hole effective masses must be known for the material in question. We use the values shown in Table S7 for the GaAs and CdTe quantum wells referred to in the main body of our paper.

TABLE S7. Dielectric constant $\epsilon$, electron effective mass $m_e$, and hole effective mass $m_h$ for GaAs and CdTe quantum wells.

| Parameter | GaAs | CdTe |
|---|---|---|
| $\epsilon$ | 13.13 [14] | 10.2 [15] |
| $m_e$ (a.u.) | 0.067 [16] | 0.096 [17] |
| $m_h$ (a.u.) | 0.34 [16] | 0.4 [17] |


[1] J. Arponen, J. Phys. C: Solid State Physics **11**, L739 (1978).
[2] N.D. Drummond and R.J. Needs, Phys. Rev. B **79**, 085414 (2009).
[3] X. Zhu, M.S. Hybertsen, and P.B. Littlewood, Phys. Rev. B **54**, 13575 (1996).
[4] X.L. Yang, S.H. Guo, F.T. Chan, K.W. Wong, and W.Y. Ching, Phys. Rev. A **43**, 1186 (1991).
[5] V. Huard, R.T. Cox, K. Saminadayar, A. Arnoult, and S. Tatarenko, Phys. Rev. Lett. **84**, 187 (2000).
[6] W.A. Goddard, III, Phys. Rev. **172**, 7 (1968).
[7] C.H. Hodges and M.J. Stott, Phys. Rev. B **7**, 73 (1973).
[8] S. Kahana, Phys. Rev. **129**, 1622 (1963).
[9] J.P. Carbotte and S. Kahana, Phys. Rev. **139**, A213 (1965).
[10] N.D. Drummond, P. López Ríos, R.J. Needs, and C.J. Pickard, Phys. Rev. Lett. **107**, 207402 (2011).
[11] T. Kato, Commun. Pure Appl. Math. **10**, 151 (1957); R.T. Pack and W.B. Brown, J. Chem. Phys. **45**, 556 (1966).
[12] N.D. Drummond, P. López Ríos, C.J. Pickard, and R.J. Needs, Phys. Rev. B **82**, 035107 (2010).
[13] S.A. Bonev and N.W. Ashcroft, Phys. Rev. B **64**, 224112 (2001).
[14] *Introduction to Solid State Physics*, C. Kittel, John Wiley and Sons Inc., Hoboken, New Jersey (2005).
[15] *Physics of semiconductors and their heterostructures*, J. Singh, McGraw-Hill, New York (1993).
[16] G. Livescu, D.A.B. Miller, D.S. Chemla, M. Ramaswamy, T.Y. Chang, N. Sauer, A.C. Gossard, and J.H. English, IEEE J. Quant. Electron. **24**, 1677 (1988).
[17] E.J. Tyrrell and J.M. Smith, Phys. Rev. B **84**, 165328 (2011).

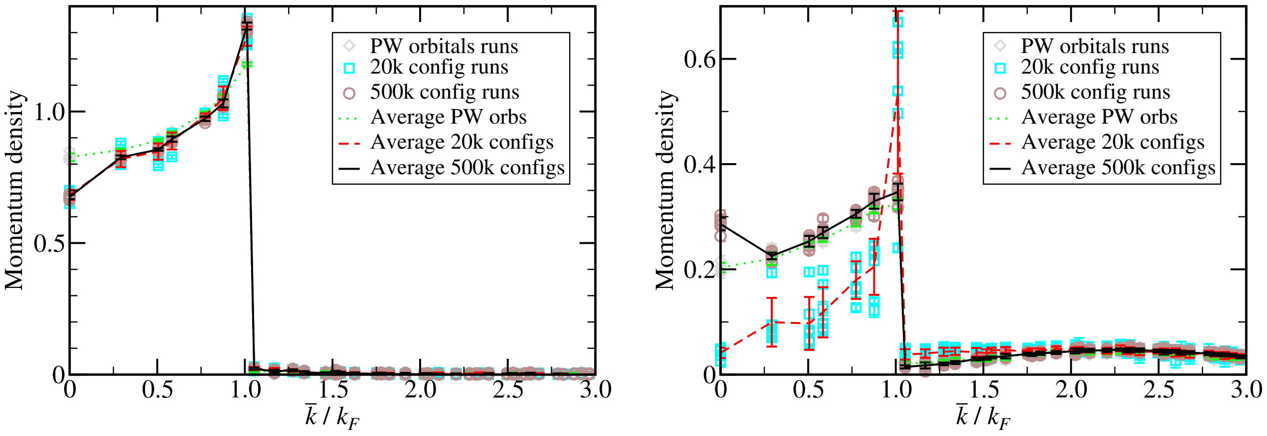


FIG. S14. Momentum densities for $m_h/m_e = 1$, $r_s = 1$ a.u. (left), and $m_h/m_e = 8$, $r_s = 6$ a.u. (right). The momentum densities were evaluated using wave function parameter sets optimized using 500,000 configurations (solid black line) and 20,000 configurations (dashed red line). The plane-wave orbital result is also shown (dotted green line), together with the individual runs that were averaged to obtain each of the three lines shown. Lines denote averaged results; symbols show the results from each independent parameter set.
